# Supplementary material for: Coupling between small polarons and ferroelectricity in BaTiO3
Source: arXiv:2503.12693 source file (2025-09-15)
Supplement: Supplementary file 1 [file Supplementary.pdf]

## Coupling between small polarons and ferroelectricity in $BaTiO_3$

Darin Joseph
*Dipartimento di Fisica e Astronomia, Universit`a di Bologna, 40127 Bologna, Italy*

Cesare Franchini
*University of Vienna, Faculty of Physics, Center for Computational Materials Science, Vienna, Austria and Dipartimento di Fisica e Astronomia, Universita` di Bologna, 40127 Bologna, Italy*

Table S1: The table represents the changes to Bond-length(BL) of polaronic unit cell and its first nearest neighbours(1NN) due to the formation of electron polarons in tetragonal $BaTiO_3$. Positive sign represents an increase and negative sign represents a decrease.

| Site type | Changes to Polaronic BL | | | % change to FE |
|---|---|---|---|---|
| | [100] | [010] | [001] | |
| Polaronic | +0.06<br>+0.06 | +0.06<br>+0.06 | +0.04<br>-0.03 | -15.6 |
| [100] 1NN | -0.07<br>- | -<br>- | +0.01<br>+0.018 | +1.6 |
| [010] 1NN | -<br>- | -0.07<br>- | +0.01<br>+0.018 | +1.6 |
| [001] 1NN | -<br>- | -<br>- | +0.017<br>-0.05 | -14.4 |
| $[00\bar{1}]$ 1NN | -<br>- | -<br>- | +0.015<br>- | -2 |

Table S2: The table represents the changes to Bond-length(BL) of polaronic unit cell and its first nearest neighbours due to the formation of electron polarons in rhombohedral $BaTiO_3$.

| Site type | Changes to Polaronic BL | | | % change to FE | | |
|---|---|---|---|---|---|---|
| | [100] | [010] | [001] | x | y | z |
| Polaronic | -0.04<br>+0.14 | -0.04<br>+0.14 | -0.04<br>+0.14 | +68 | +68 | +68 |
| [100] 1NN | -0.15<br>+0.08 | +0.01<br>- | +0.01<br>- | -85 | +1 | +1 |

| | | | | | | |
|---|---|---|---|---|---|---|
| $[\bar{1}00]$ 1NN | -0.06<br>+0.03 | -<br>- | -<br>- | -33 | 0 | 0 |
| [010] 1NN | +0.01<br>- | -0.15<br>+0.08 | +0.01<br>- | +1 | -85 | +1 |
| $[0\bar{1}0]$ 1NN | -<br>- | -0.06<br>+0.03 | -<br>- | 0 | -33 | 0 |
| [001] 1NN | +0.01<br>- | +0.01<br>- | -0.15<br>+0.08 | +1 | +1 | -85 |
| $[00\bar{1}]$ 1NN | -<br>- | -<br>- | -0.06<br>+0.03 | 0 | 0 | -33 |

Table S3: The table represents the changes to Bond-length(BL) of polaronic unit cell and its first nearest neighbours and second nearest neighbours(2NN) due to the formation of hole polarons in tetragonal $BaTiO_3$.

| Site type | Changes to Polaronic BL | | | % change to FE | | |
|---|---|---|---|---|---|---|
| | [100] | [010] | [001] | x | y | z |
| [100] 1NN | +0.08<br>-0.08 | -0.02<br>-0.02 | -<br>- | +15 | 0 | 0 |
| $[\bar{1}00]$ 1NN | -0.08<br>+0.08 | -0.02<br>-0.02 | -<br>- | +15<br>(opp. Direction) | 0 | 0 |
| [100] 2NN | -0.01<br>- | -<br>- | -0.01<br>-0.01 | -0.8 | 0 | 0 |
| [010] 2NN | -<br>-0.01 | -0.01<br>+0.03 | -<br>-0.01 | +1 | +4 | -1 |
| $[0\bar{1}0]$ 2NN | -<br>-0.01 | +0.03<br>-0.01 | -<br>-0.01 | +1 | -4 | -1 |
| [001] 2NN | -<br>- | -<br>- | -<br>+0.02 | 0 | 0 | +6 |

| | | | | | | |
|---|---|---|---|---|---|---|
| $[00\bar{1}]$ 2NN | -<br>- | -<br>- | -<br>-0.008 | 0 | 0 | -3 |

Table S4: The table represents the changes to Bond-length(BL) of polaronic unit cell and its first nearest neighbours and second nearest neighbours(2NN) due to the formation of hole polarons in rhombohedral $BaTiO_3$.

| Site type | Changes to Polaronic BL | | | % change to FE | | |
|---|---|---|---|---|---|---|
| | [100] | [010] | [001] | x | y | z |
| [100] 1NN | -0.01<br>+0.01 | -0.02<br>-0.006 | -0.02<br>-0.01 | -10 | +11 | -5 |
| $[\bar{1}00]$ 1NN | -0.21<br>+0.21 | -0.01<br>-0.01 | -0.02<br>-0.01 | -49<br>(opp. Direction) | 0 | -5 |
| [100] 2NN | -0.1<br>+0.10 | -<br>-0.01 | -<br>-0.018 | -74 | +4 | +4 |
| [010] 2NN | -0.01<br>-0.008 | -0.02<br>+0.02 | -0.01<br>+0.008 | 0 | -17 | -6 |
| [010]2NN | -<br>- | +0.02<br>-0.008 | -<br>- | 0 | +12 | 0 |
| $[0\bar{1}0]$ 2NN | -<br>- | +0.01<br>- | -<br>- | 0 | +3 | 0 |
| $[0\bar{1}0]$ 2NN | -<br>- | -<br>- | -<br>- | 0 | 0 | 0 |

| | | | | | | |
|---|---|---|---|---|---|---|
| [001] 2NN | -<br>- | -<br>- | +0.03<br>-0.006 | 0 | 0 | +14 |
| [001] 2NN | -<br>- | -<br>- | +0.03<br>-0.007 | 0 | 0 | +14 |
| $[00\bar{1}]$ 2NN | -<br>- | -<br>- | -<br>+0.01 | 0 | 0 | -3 |
| $[00\bar{1}]$ 2NN | -<br>- | -<br>- | -<br>+0.01 | 0 | 0 | 0 |
